# Supplementary material for: Variable selection in high-dimensional logistic regression models using a whitening approach
Source: arXiv:2206.14850 source file (2022-06-29)
Supplement: Supplementary file 1 [file supp.tex]

\newpage
Suppose the new tranformation $\widetilde{\bX}=\bX\bS$, we hope that $$\widetilde{\bX}^{T}H\widetilde{\bX}=I_{p}$$
$\widetilde{\bX}^{T}H\widetilde{\bX}=(\bX\bS)^{T}H(\bX\bS)=\bS^{T}(\bX^{T}H\bX)\bS$. If $E(\bX^{T}H\bX)=\Check{\bSigma}$ then $\bS=\Check{\bSigma}^{-1/2}$\\

\textbf{Solution 1}

\begin{enumerate}
    \item $\widetilde{\bX}=H^{-1/2}\bX\bSigma^{-1/2}$ and $\widetilde{\bbeta} = \bSigma^{1/2}\bbeta$
\end{enumerate}
\textcolor{red}{model changed}\\

\textbf{Solution 2}
\begin{enumerate}
    \item note $\Check{\bX}=H^{1/2}\bX$
    \item estimate the covariance matrix of $\Check{\bX}$, note as $\Check{\bSigma}$
    \item $\widetilde{\bX}=\bX\Check{\bSigma}^{-1/2}$ and $\widetilde{\bbeta} = \Check{\bSigma}^{1/2}\bbeta$
\end{enumerate}
\textcolor{red}{biased estimation of $\Check{\bSigma}$}\\

\textbf{Solution 3}
\begin{enumerate}
    \item make approximation on H (all elements equal to 0.25, prob=0.5)
    \item $\widetilde{\bX}=\bX\bSigma^{-1/2}$ and $\widetilde{\bbeta} = \bSigma^{1/2}\bbeta$
\end{enumerate}
\textcolor{red}{potential drawbacks on approximation}

\newpage
Suppose $\widetilde{\bX}=\bX\Sigma^{-1/2}$, and let
\begin{equation}
    \rho_{jk}=\frac{1}{n}\sum_{i=1}^{n}\widetilde{\bX}_{ij}\widetilde{\bX}_{ik}, 1\leq j,k\leq p
\end{equation}

then $\mathbb{E}(\rho_{jk})=0 (k\neq j)$. In logistic regression, let

\begin{equation}
    \widetilde{\rho}_{jk}=\frac{1}{n}\sum_{i=1}^{n}\eta_{ii}\widetilde{\bX}_{ij}\widetilde{\bX}_{ik}, 1\leq j,k\leq p
\end{equation}
where $\eta_{ii}=p(X^{(i)})/(1-p(X^{(i)}))$ and $p(X^{(i)})=Pr(y_{i}=1|X^{(i)})$ the probability for observation $i$, then $\eta_{ii}\leq0.25$ for all $i$. Therefore
\begin{align*}
\widetilde{\rho}_{jk}&\leq \frac{0.25}{n}\sum_{i=1}^{n}\widetilde{\bX}_{ij}\widetilde{\bX}_{ik}\\
         &=0.25\rho_{jk}
\end{align*}
